# Supplementary material for: Keys to Better Image Inpainting: Structure and Texture Go Hand in Hand
Source: arXiv:2208.03382 source file (2022-12-02)
Supplement: Supplementary file 1 [file ffc.tex]

\begin{comment}
\section{Fast Fourier Convolutions}
\label{sec:ffc}

\begin{figure}[ht!]
\centering
\includegraphics[width=0.9\linewidth]{supplementary/graphics/ffc.pdf}
\caption{\textbf{FFC Layer.} It uses the Spectral Transform module in the global branch to account for the global context similar to LaMa~\cite{lama}}
\label{fig:ffc}
\end{figure}

\noindent
FFC \cite{ffc} is based on a channel-wise fast Fourier transform (FFT) \cite{fft}. The FFC layer splits channels into two branches (\cref{fig:ffc}): a) local branch uses conventional convolutions to capture the spatial details, and b) global branch that uses real FFT to account for global context in the spectral domain. The local branch learns the features from the pixels in the neighborhood using the convolutional kernels (limited receptive field). The global branch uses a Spectral Transform module to consider the global structure and capture the long-range context (enlarge the receptive field). Finally, the outputs of the local (\emph{i}) and global (\emph{ii}) branches are stacked together.

The spectral transform uses two Fourier Units (FU) to capture the global and semi-global information. The left Fourier Unit (FU) in \cref{fig:ffc} takes models the global context. On the other hand, the Local Fourier Unit (LFU) on the right side in \cref{fig:ffc} takes in a quarter of the channels and focuses on the semi-global information in the image.

A Fourier Unit mainly breaks down the spatial structure into image frequencies using a Real FFT2D operation, a convolution operation in the frequency domain and finally recovering the structure using an Inverse FFT2D operation.

% \begin{equation}
%     \begin{split}
%          \textit{(a)} \ & \text{Apply Real FFT2d. Concatenate real and imaginary parts:} \\
%          & \quad \text{Real FFT2d} \Longrightarrow  \mathbb{R}^{H\times W\times C}\to\mathbb{C}^{H\times \frac{W}{2} \times C} \\
%          & \quad \text{Complex To Real} \Longrightarrow \mathbb{C}^{H\times \frac{W}{2}\times C}\to\mathbb{R}^{H\times \frac{W}{2} \times 2C} \\
%         \textit{(b)} \ & \text{Apply ReLU + Conv in the frequency domain:} \\
%         & \quad \textit{ReLU}\circ\textit{Conv1}\!\!\times\!\!\textit{1} \Longrightarrow \mathbb{R}^{H\times \frac{W}{2} \times 2C}\to\mathbb{R}^{H\times \frac{W}{2} \times 2C} \\
%         \textit{(c)} \ & \text{Apply inverse FFT2d to recover global spatial structures:} \\
%         & \quad \text{Real To Complex} \Longrightarrow \mathbb{R}^{H\times \frac{W}{2} \times 2C}\to\mathbb{C}^{H\times \frac{W}{2} \times C} \\
%         & \quad \text{Inverse Real FFT2d} \Longrightarrow \mathbb{C}^{H\times \frac{W}{2} \times C} \to \mathbb{R}^{H\times W\times C} \\
%     \end{split}
%     \label{eq:ffc}
% \end{equation}
\end{comment}
