# Supplementary material for: Keys to Better Image Inpainting: Structure and Texture Go Hand in Hand
Source: arXiv:2208.03382 source file (2022-12-02)
Supplement: Supplementary file 2 [file 512.tex]

\begin{tabular}{lcc}
\toprule
{\textbf{Method}} & {FID$\downarrow$ } & {LPIPS$\downarrow$ } \\
\midrule
CoModGAN (official)~\cite{comodgan} & $2.32$ & $0.045$ \\
LaMa (official)~\cite{lama} & $2.00$ & $0.040$ \\
%Big-LaMa~\mcite{26} & $\mathbf{1.77}$ & $\mathbf{0.037}$ \\
%\midrule
FcFGAN (ours) & $2.06$ & $0.041$ \\

\bottomrule
\end{tabular}
