# Supplementary material for: Keys to Better Image Inpainting: Structure and Texture Go Hand in Hand
Source: arXiv:2208.03382 source file (2022-12-02)
Supplement: Supplementary file 3 [file user_study.tex]

\begin{tabular}{lcc}
\toprule
{\textbf{Method}} & \textbf{User Study (CoModGAN vs Ours)} \\
\midrule
CoModGAN (official)~\cite{comodgan} & 21.33\% \\
FcFGAN (ours) & \textbf{61.33\%} \\
\midrule
{\textbf{Method}} & \textbf{User Study (LaMa vs Ours)} \\
\midrule
LaMa (official)~\cite{lama} & 39.33\% \\
FcFGAN (ours) & \textbf{48.67\%} \\

\bottomrule
\end{tabular}
